# Supplementary material for: HRP: Human Affordances for Robotic Pre-Training
Source: arXiv:2407.18911 source file (2024-07-26)
Supplement: Supplementary file 1 [file supp.tex]

\documentclass[conference]{IEEEtran}
\usepackage{times}

% numbers option provides compact numerical references in the text. 
\usepackage[numbers]{natbib}
\usepackage{multicol}

\usepackage{graphics,graphicx,caption,float,subcaption,booktabs,xcolor,multirow,array,color,ifthen,tabu,colortbl,dblfloatfix,url,xparse,mathtools,patchcmd,algorithm,algorithmic,amssymb,xspace,nicefrac,microtype,amsmath,amsfonts,bm,ragged2e,tikz,stackengine,etoolbox,xpatch,enumerate,xstring,setspace,tabularx,makecell,changepage,cuted,titlesec,wrapfig,tcolorbox, sidecap, xspace, dsfont, algorithm, listings}

\usepackage[pagebackref=true,breaklinks=true,colorlinks=true,bookmarks=false,citecolor=blue]{hyperref}

\pdfinfo{
   /Author (Homer Simpson)
   /Title  (Robots: Our new overlords)
   /CreationDate (D:20101201120000)
   /Subject (Robots)
   /Keywords (Robots;Overlords)
}

\definecolor{msgreen}{rgb}{0.19215686,  0.63921569,  0.32941176}
\definecolor{msred}{rgb}{0.87058824,  0.17647059,  0.14901961}
\definecolor{msblue}{rgb}{0.19215686,  0.50980392,  0.74117647}

\begin{document}

% paper title
\title{HRP: Human Affordances for Robotic Pre-Training}

% You will get a Paper-ID when submitting a pdf file to the conference system
\author{Author Names Omitted for Anonymous Review. Paper-ID 337}

\appendix
\input{sections/99-appendix}

\bibliographystyle{plainnat}
\bibliography{references}

\end{document}
